# Supplementary material for: Evaluating Perceived Usefulness and Ease of Use of CMMN and DCR
Source: arXiv:2103.11218 source file (2021-05-03)
Supplement: Supplementary file 1 [file Section06_AppendixA.tex]

\section{Appendix A. Questionaire}\label{Sec:AppendixA}

Here, you can find a part of the questionnaire used in both Survey 1 and Survey 2 that is used in this paper.
We omitted the qualitative questions in which we asked about participants' comments - as they are outside the scope of this paper.
Participants could choose answers based on scales as listed here: 
\textit{extremely likely}, 
\textit{quite likely}, 
\textit{slightly likely}, 
\textit{neither likely nor unlikely}, 
\textit{slightly unlikely}, 
\textit{quite unlikely}, 
\textit{extremely unlikely}.
These options (with the specified order) are mapped to an ordinal scale.
The \textit{extremely likely} option is mapped to 7 and \textit{extremely unlikely} option is mapped to 1.

Here is the template for the questions that we asked to measure the \textit{perceived usefulness} and \textit{perceived ease of use} of DCR and CMMN.
In this template, we replaced the \textit{\{languague\}} with DCR or CMMN for the questions that we asked for each of these languages.
The questions are defined based on the technology acceptance model.

\subsection{Template for perceived usefulness}

\begin{itemize}
	\item Using \{languague\} in this experience enabled me to model business processes more quickly.
	\item Using \{languague\} in this experience improved my performance when modeling business processes.
	\item Using \{languague\} in this experience increased my productivity when modeling business processes.
	\item Using \{languague\} in this experience enhanced my effectiveness in modeling business processes.
	\item Using \{languague\} in this experience made it easier for me to model business processes. 
	\item I found \{languague\} useful in this experience.
\end{itemize}

\subsection{Template for perceived ease of use}

\begin{itemize}
	\item Learning how to use \{languague\} was easy for me.
	\item I found it easy to get \{languague\} to do what I wanted to do.
	\item I found \{languague\} understandable and clear.
	\item I found \{languague\} flexible to be used in modeling business processes.
	\item It was easy for me to become skillful at using \{languague\}.
	\item I found \{languague\} easy to use.
\end{itemize}
